# Supplementary material for: Gyrokinetic Continuum Simulation of Turbulence in Open-Field-Line Plasmas
Source: arXiv:1708.07283 source file (2017-08-24)
Supplement: Supplementary file 1 [file code.tex]

\chapter{Supplementary Code\label{ch:supplementary-code}}

The code in this section makes extensive use of a
Lua function \texttt{runUpdater}, which we define as
\begin{lstlisting}[language={[5.2]Lua}]
function runUpdater(updater, currTime, timeStep, inpFlds, outFlds)
   updater:setCurrTime(currTime)
   if inpFlds then
      updater:setIn(inpFlds)
   end
   if outFlds then
      updater:setOut(outFlds)
   end
   return updater:advance(currTime+timeStep)
end
\end{lstlisting}

\section{Limiter Bias Modifications}
To model limiter biaising in the 3D2V LAPD simulations of Section \ref{ch:lapd},
a 3D potential field is created in the Lua script and set to have the value 0 along field lines
that do not intersect the biasable limiter and $V_{\mathrm{bias}}$ along field lines that do.
The following code block creates the bias field $\phi_\mathrm{bias}$, which is the variable \texttt{phiOffset}.

\begin{lstlisting}[language={[5.2]Lua}]
initPhiOffset = Updater.EvalOnNodes3D {
  onGrid = grid_3d,
  basis = basis_3d,
  shareCommonNodes = false,
  evaluate = function(x,y,z,t)
    local r = math.sqrt(x^2 + y^2)
    if r >= r_s then
      return V_bias
    else
      return 0
    end
  end
}
-- offset potential for sheath bc
phiOffset = DataStruct.Field3D {
   onGrid = grid_3d,
   numComponents = basis_3d:numNodes(),
   ghost = {1, 1},
}
runUpdater(initPhiOffset, 0, 0, {}, {phiOffset})
\end{lstlisting}

The \texttt{phiOffset} field is then combined with the electrostatic potential that is
the solution of the gyrokinetic Poisson equation (labeled as \texttt{phi3d}) into the
sheath potential field \texttt{phiSheath}, which is used in the sheath-model boundary conditions.
The following code shows how this procedure is implemented in the function that applies
boundary conditions to the distribution functions.

\begin{lstlisting}[language={[5.2]Lua}]
function applyBcToDistF(tCurr, myDt, fElc, fIon, phiIn)
  fIon:sync()
  fElc:sync()
  -- apply zero inflow boundary conditions in z to ions
  runUpdater(bcLowerZIon, tCurr, myDt, {}, {fIon})
  runUpdater(bcUpperZIon, tCurr, myDt, {}, {fIon})
  -- apply zero inflow boundary conditions in z to electrons
  runUpdater(bcLowerZElc, tCurr, myDt, {}, {fElc})
  runUpdater(bcUpperZElc, tCurr, myDt, {}, {fElc})
  -- compute potential for sheath bc
  phiSheath:combine(1.0, phiIn, -1.0, phiOffset)
  -- apply biased sheath boundary conditions to electron distribution
  -- function
  runUpdater(biasedSheathElcCalc, tCurr, myDt, {phiSheath,
    hamilDerivKeElc}, {fElc})
  -- apply biased sheath boundary conditions to ion distribution 
  -- function
  runUpdater(biasedSheathIonCalc, tCurr, myDt, {phiSheath,
    hamilDerivKeIon}, {fIon})
  -- sync cells in distribution function 
  fElc:sync()
  fIon:sync()
end
\end{lstlisting}
