# Supplementary material for: Gyrokinetic Continuum Simulation of Turbulence in Open-Field-Line Plasmas
Source: arXiv:1708.07283 source file (2017-08-24)
Supplement: Supplementary file 2 [file post-processing.tex]

\chapter{Post-Processing Methods}
In this section, we document the post-processing methods employed elsewhere in this thesis.
\hl{Plotting, Fourier transforms, correlation functions}
